# Supplementary material for: Unsupervised Learning from Video with Deep Neural Embeddings
Source: arXiv:1905.11954 source file (2020-03-10)
Supplement: Supplementary file 1 [file supplementary.tex]

\documentclass[10pt,twocolumn,letterpaper]{article}

\usepackage[utf8]{inputenc} % allow utf-8 input
\usepackage[T1]{fontenc}    % use 8-bit T1 fonts
\usepackage{url}            % simple URL typesetting
\usepackage{booktabs}       % professional-quality tables
\usepackage{amsfonts}       % blackboard math symbols
\usepackage{nicefrac}       % compact symbols for 1/2, etc.
\usepackage{microtype}      % microtypography
\usepackage{xcolor}
\usepackage{bbm}
\usepackage{amsmath}
\usepackage{xspace}
\usepackage{graphicx}
\usepackage{bm}
\usepackage{multicol}
\usepackage{multirow}
\usepackage[font=small]{caption} 
\captionsetup[table]{skip=10pt}

\input{sections/new_commands.tex}
\usepackage[pagebackref=true,breaklinks=true,letterpaper=true,colorlinks,bookmarks=false]{hyperref}

\begin{document}

%%%%%%%%% TITLE
\title{Supplementary Material}
\date{}
\maketitle

\input{sections/appendix.tex}

{\small
\bibliographystyle{ieee_fullname}
\bibliography{references}
}

\end{document}
